# Supplementary material for: Disentangled and Controllable Face Image Generation via 3D Imitative-Contrastive Learning
Source: arXiv:2004.11660 source file (2020-09-04)
Supplement: Supplementary file 1 [file supplementary.pdf]

# Disentangled and Controllable Face Image Generation via 3D Imitative-Contrastive Learning
## *(Supplementary Material)*

Yu Deng[*1,2] Jiaolong Yang[2] Dong Chen[2] Fang Wen[2] Xin Tong[2]
[1]Tsinghua University [2]Microsoft Research Asia
{t-yudeng,jiaoyan,doch,fangwen,xtong}@microsoft.com

## I. More Implementation Details

**VAE structure.** We use the same VAE structure for identity $\alpha$, expression $\beta$, illumination $\gamma$, and pose $\theta$ in $\lambda$ space. They have three hidden layers for both encoder and decoder. Dimensions of hidden layers in each VAE are 512, 256, 128, and 32 respectively. We use ReLU as the activation layer.

**Latent variable dimensions.** The $z$-space variable dimensions are empirically set to 128, 32, 16, and 3 for $z_1$ to $z_4$, respectively, and the dimensions of corresponding latent variable in $\lambda$-space are 160, 64, 27, and 3. The dimension of the additional noise $z_5$ is 32.

**Training details.** We train the $\lambda$-space VAEs following the schedule of [1] where we only adopt the first stage. For StyleGAN [3], we follow the standard training procedure of the original method on the FFHQ dataset except that we 1) remove the normalization operation for input latent variable layer, 2) discard the style-mixing strategy, and 3) train up to image resolution of $256 \times 256$ due to time constraint.

The StyleGAN training uses a progressive growing strategy [2] where the image resolution gradually increases. It is difficult to directly apply our imitative losses when the resolution is very small and image quality is poor. So when the resolution $\leq 32 \times 32$, we simply use an average $l_1$ pixel loss between the face regions of generated images and rendered ones with its weight set to 20. The adversarial loss weight is set to 1 throughout the training process. When the resolution grows to $64 \times 64$, we discard the pixel loss and apply our imitative losses described in the main paper. We train the network until seeing $15M$ real images to obtain reasonable imitation, with loss weights set as $w_{l_I^{id}} = 3$, $w_{l_I^{lm}} = 500$, $w_{l_I^{sh}} = 10$, and $w_{l_I^{cl}} = 20$. Then we add the contrastive losses and train the network up to seeing $20M$ real images with loss weights set as $w_{l_C^{ex}} = 10$, $w_{l_C^{il_1}} = 10$, and $w_{l_C^{il_2}} = 20$. The balancing weight $\omega$ in $l_C^{il_1}$ is set to 1000. During this period, the imitative loss weight $w_{l_I^{lm}}$ is reduced to 100 and others remain unchanged. Note that these loss weights and other hyper-parameters are not carefully tuned.

## II. More Generation Results

In Figure V and Figure VI, we show more generation results of *DiscoFaceGAN*. Similar to results presented in the main paper, we are able to randomly generate face images with a large variant of identities with diverse poses, illumi-nation conditions and facial expressions. The variations of identity, expression, pose and illumination are highly disen-tangled with each other. Precisely control can be achieved for expression, illumination and pose using the parametric model coefficients.

## III. Latent Space Interpolation

In Figure VII, we show some results of latent space interpolation. Since our model learns a disentangled latent space, we can interpolate each factor in the $\lambda$ space independently. When a certain factor is changing, the corresponding attributes in generated images are changing continuously and smoothly, while attributes related to other factors remain unchanged.

## IV. Attribute-Preserving Truncation Trick

In StyleGAN [3], a truncation trick is used to improve the generation quality of the model. Given a latent code $w$ in $\mathcal{W}$ space, we can move it towards a center by $w' = w + (1 - \psi)(\bar{w} - w)$, where $\bar{w}$ is the empirical average center in the $\mathcal{W}$ space, and $\psi < 1$. However, naively applying the truncation trick may change all image attributes controlled by the factors in the $\lambda$ space, whereas we hope to improve the generation quality of the identities while keeping expression, illumination and pose unchanged. Therefore, we propose an attribute-preserving truncation trick based on the latent space properties described in Section 5.1 of the main paper. Specifically, we compute an empiri-

[*]This work was done when Yu Deng was an intern at MSRA.

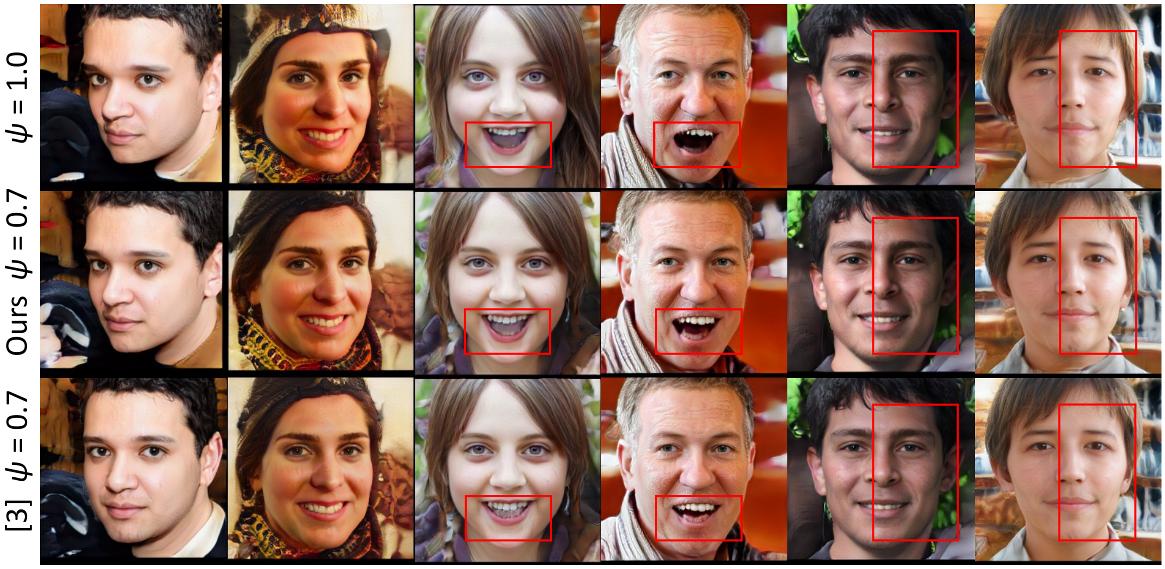


Figure I: Our attribute-preserving truncation trick improves the generation quality meanwhile maintains the pose (first two columns), expression (middle two columns), and illumination (last two columns) of the generated images. The original truncation trick in [3] cannot preserve these attributes.

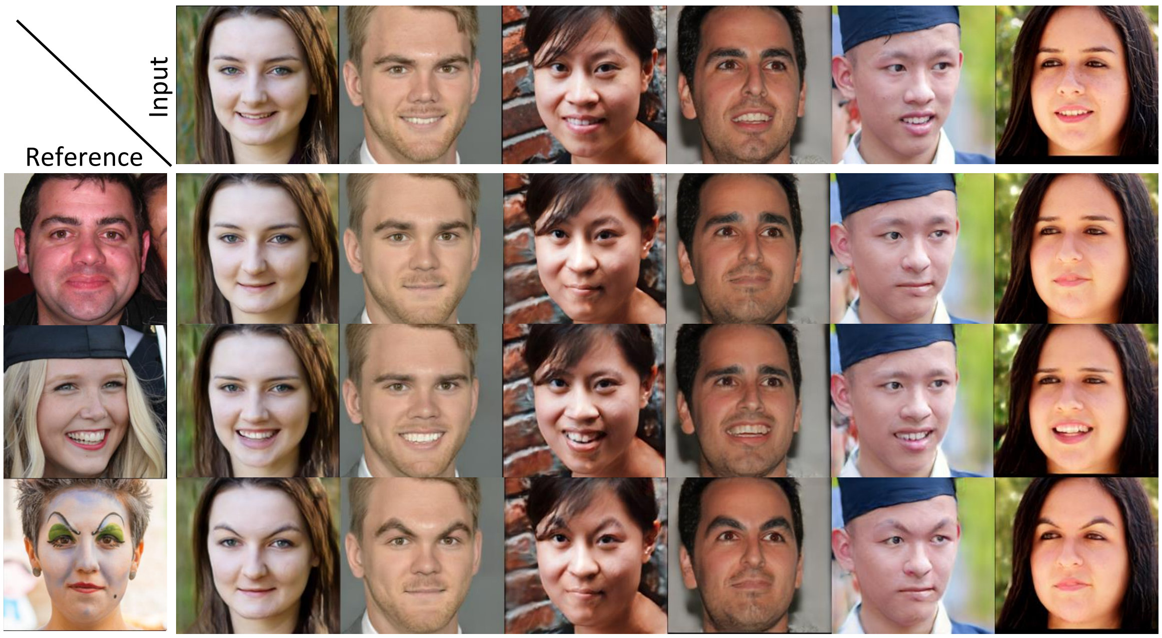


Figure II: Real image expression transfer results.

cal center $\bar{w}_\alpha = \mathbb{E}_\alpha[w(\alpha, u_{\{j\}} = 0)]$ in the $\mathcal{W}$ space with expression, illumination, and pose set to 0. Then, given a latent code $w(\alpha = a, u_{\{j\}})$, we change it with $w' = w(\alpha = a, u_{\{j\}}) + (1-\psi)(\bar{w}_\alpha - w(\alpha = a, u_{\{j\}} = 0))$. Figure I compares the original truncation trick and ours.

# V. Real Image Editing

In Section 5.2 of the main paper, we have presented some results of pose and lighting modification of real images. In Fig. II, we further show some typical results from our method in an expression transfer task. As can be seen, our method successfully transfers the desired expressions to different subjects under various poses and lighting conditions.

# VI. Analysis of Image Generation

Since we can flexibly control the generation with disentangled factor variations, we use our method to analyze image generation process of StyleGAN. We provide a stage-

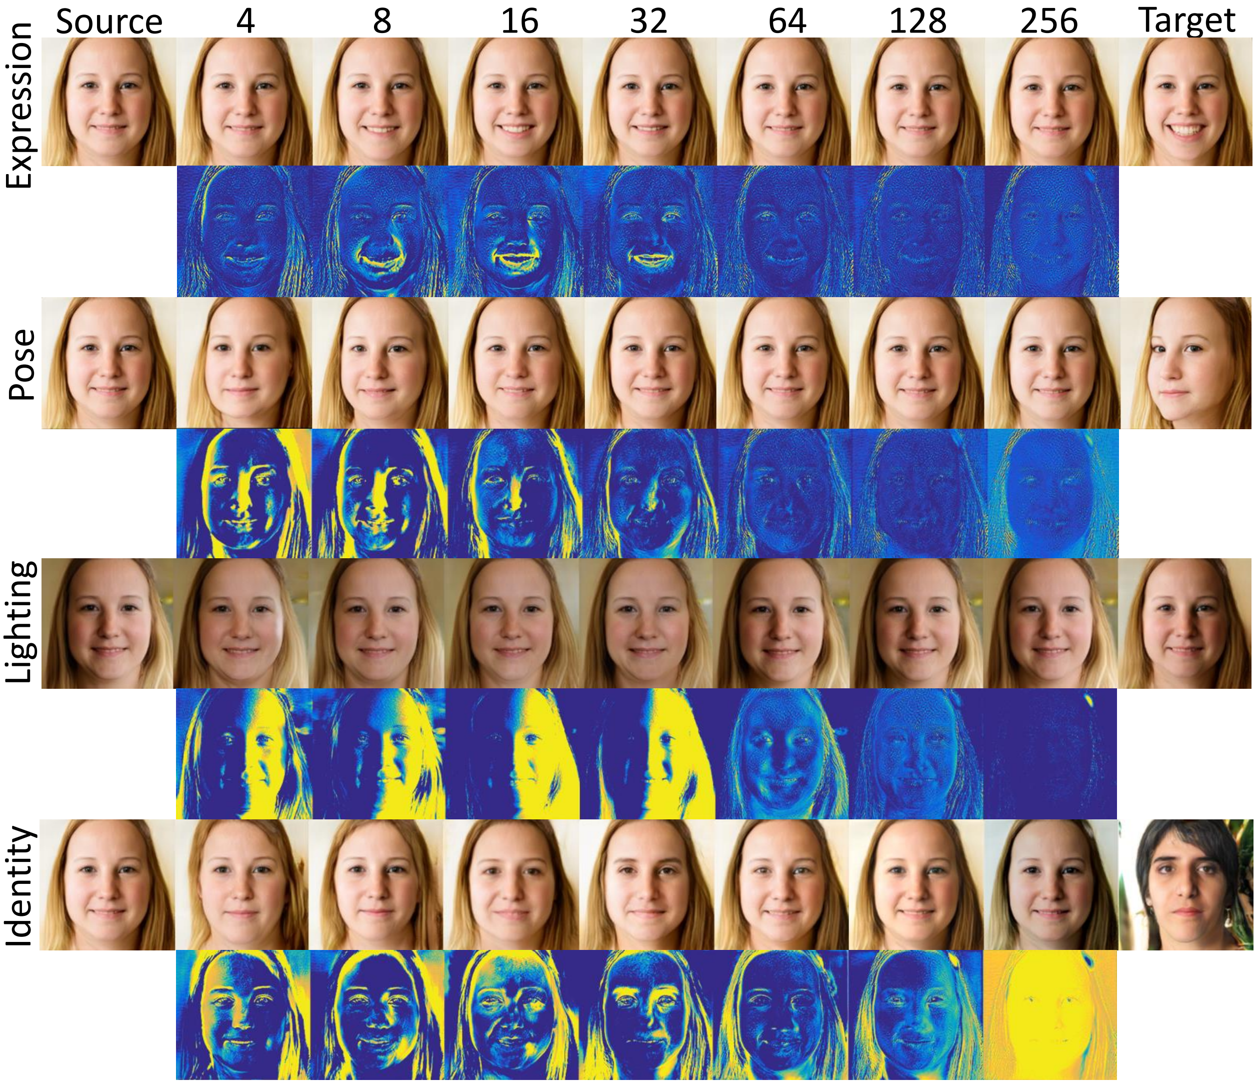


Figure III: Generation results of a $256 \times 256$-resolution StyleGAN when changing the parameters of AdaIN layers for each stage. The heatmaps show the color difference between the generated images and the original source image.

by-stage visualization of the impacts on pose, expression, lighting and identity generation. Given an image $x_s$ generated by $\lambda_s$, we replace the corresponding $w_s$ vector in the $\mathcal{W}$ space with $w_t$ for the two AdaIN layers at each generation stage (spatial resolution), where $w_t$ comes from another $\lambda_t$ which differs from $\lambda_s$ at one factor. Changes on the generated image therefore reflect the impact of each stage on the factor of interest, and Figure III shows one example.

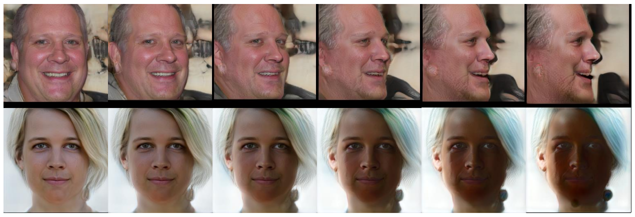

Figure IV: Quality of the generated face images decreases when input factors are out of the distribution of the real image training set.

## VII. Limitations

We have demonstrated the effectiveness of our model on disentangled and controllable face image generation. Still, our model has some limitations. Figure IV shows that degraded generation quality of the model under extreme pose and lighting. This is a common out-of-domain issue, resolving which would require using training images with a wider range of distribution beyond FFHQ. In addition, we cannot achieve the control over detailed facial expressions and eye gaze due to the limited ability of 3DMM.

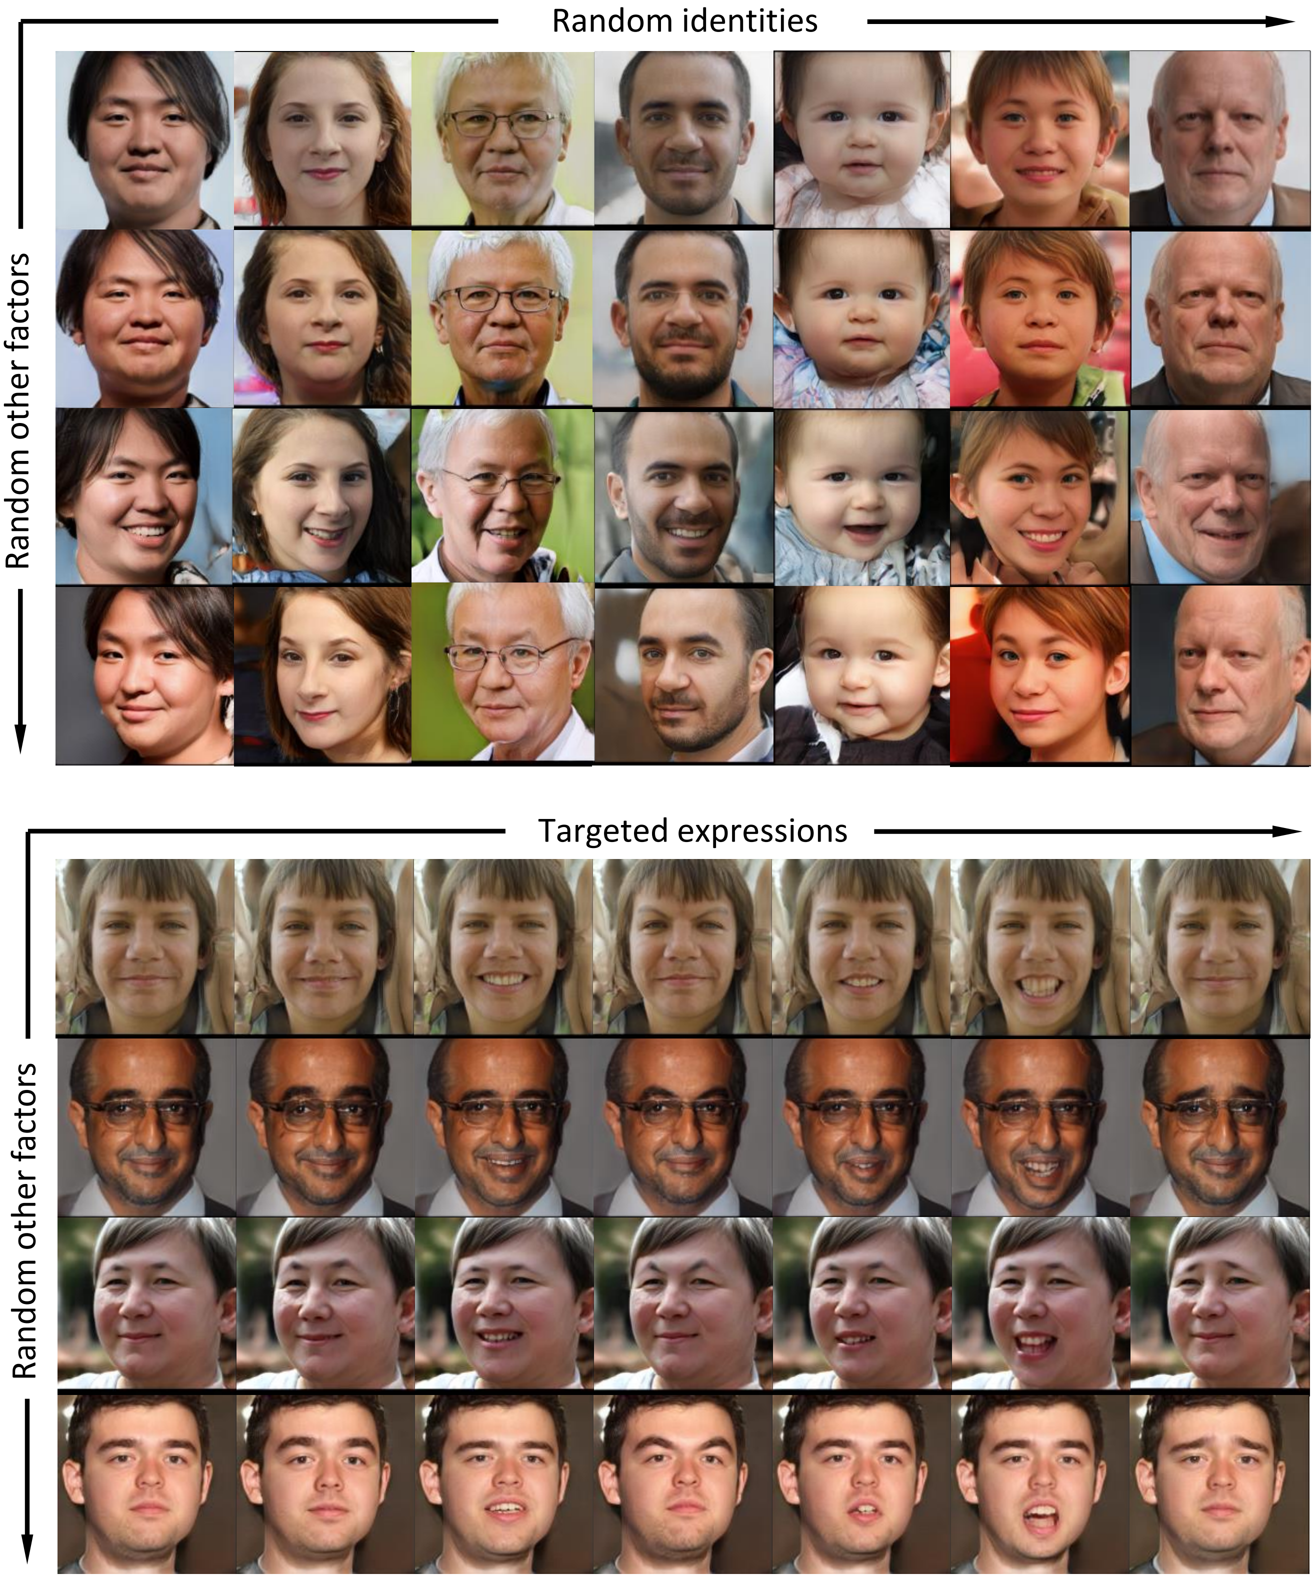


Figure V: More face images generated by our *DiscoFaceGAN*. As shown in the figures, the variations of identity, expression, pose and illumination are highly disentangled, and we can precisely control expression, illumination and pose.

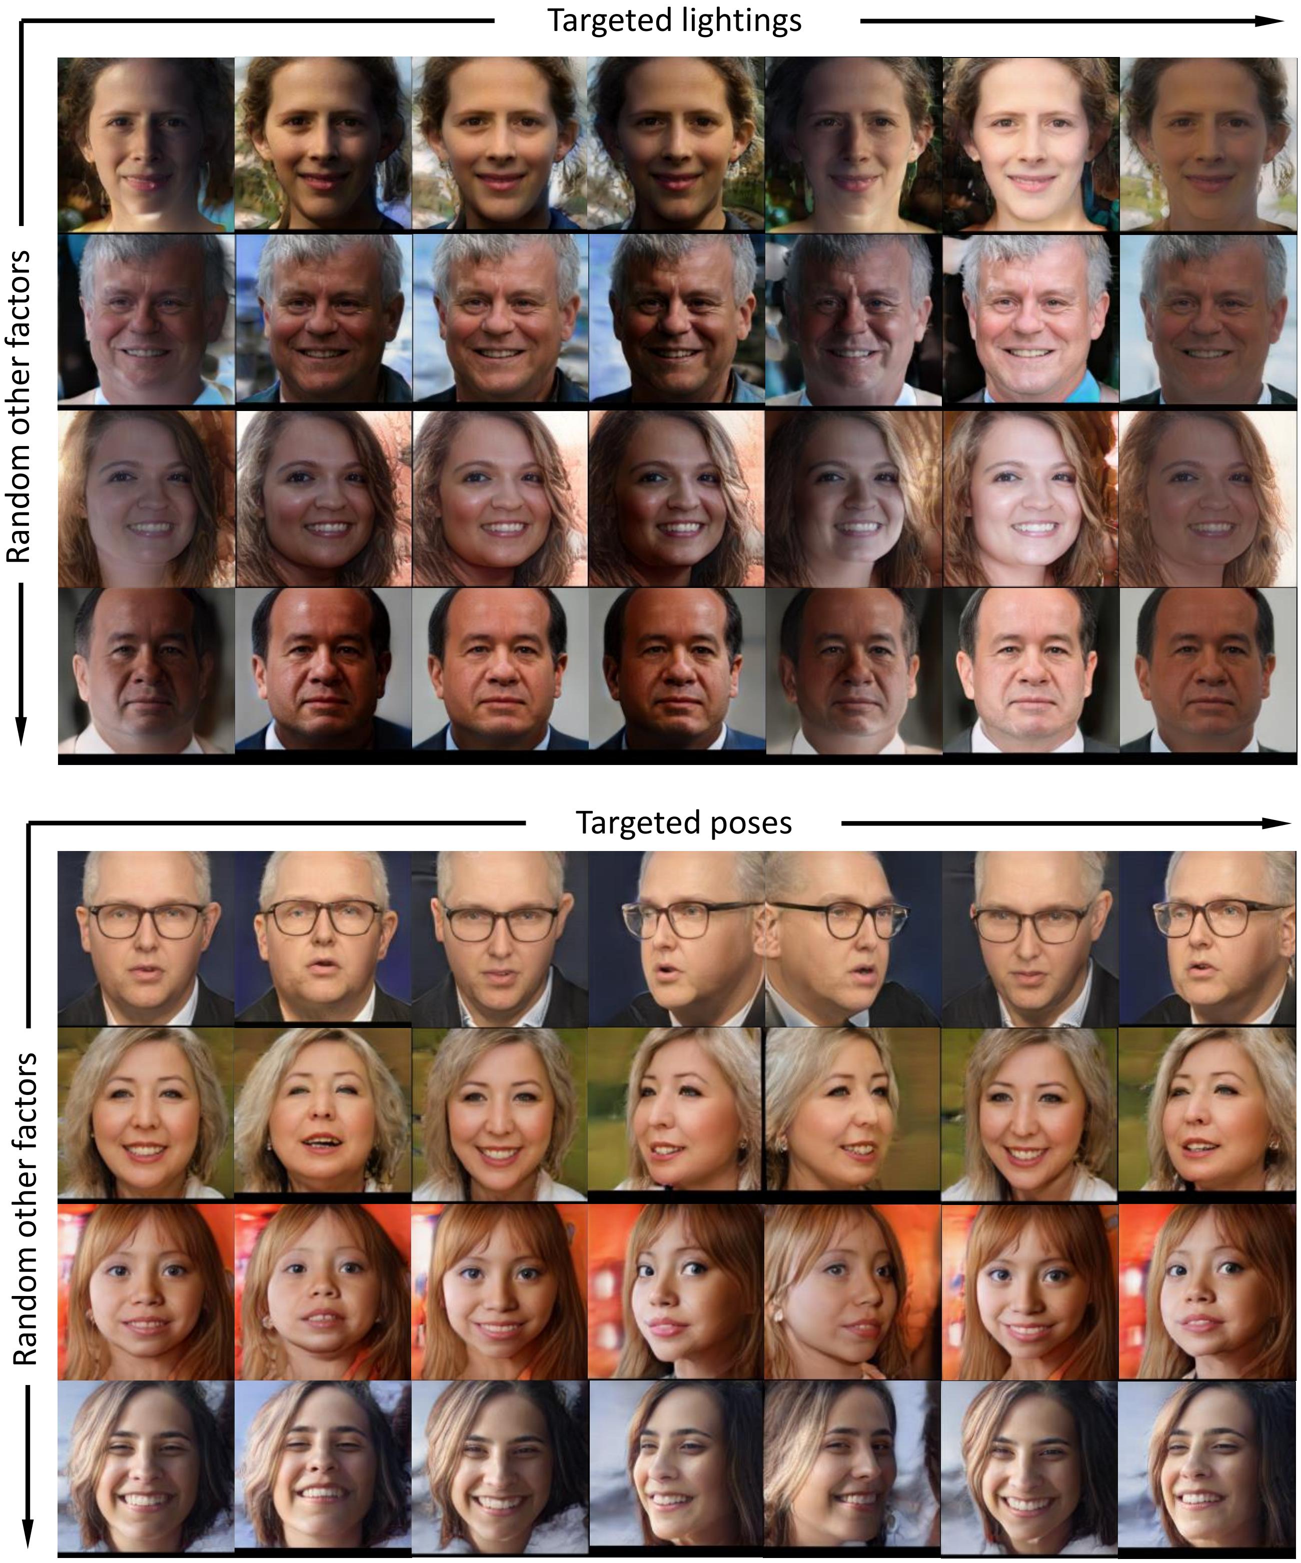


Figure VI: More face images generated by our *DiscoFaceGAN*. As shown in the figures, the variations of identity, expression, pose and illumination are highly disentangled, and we can precisely control expression, illumination and pose.

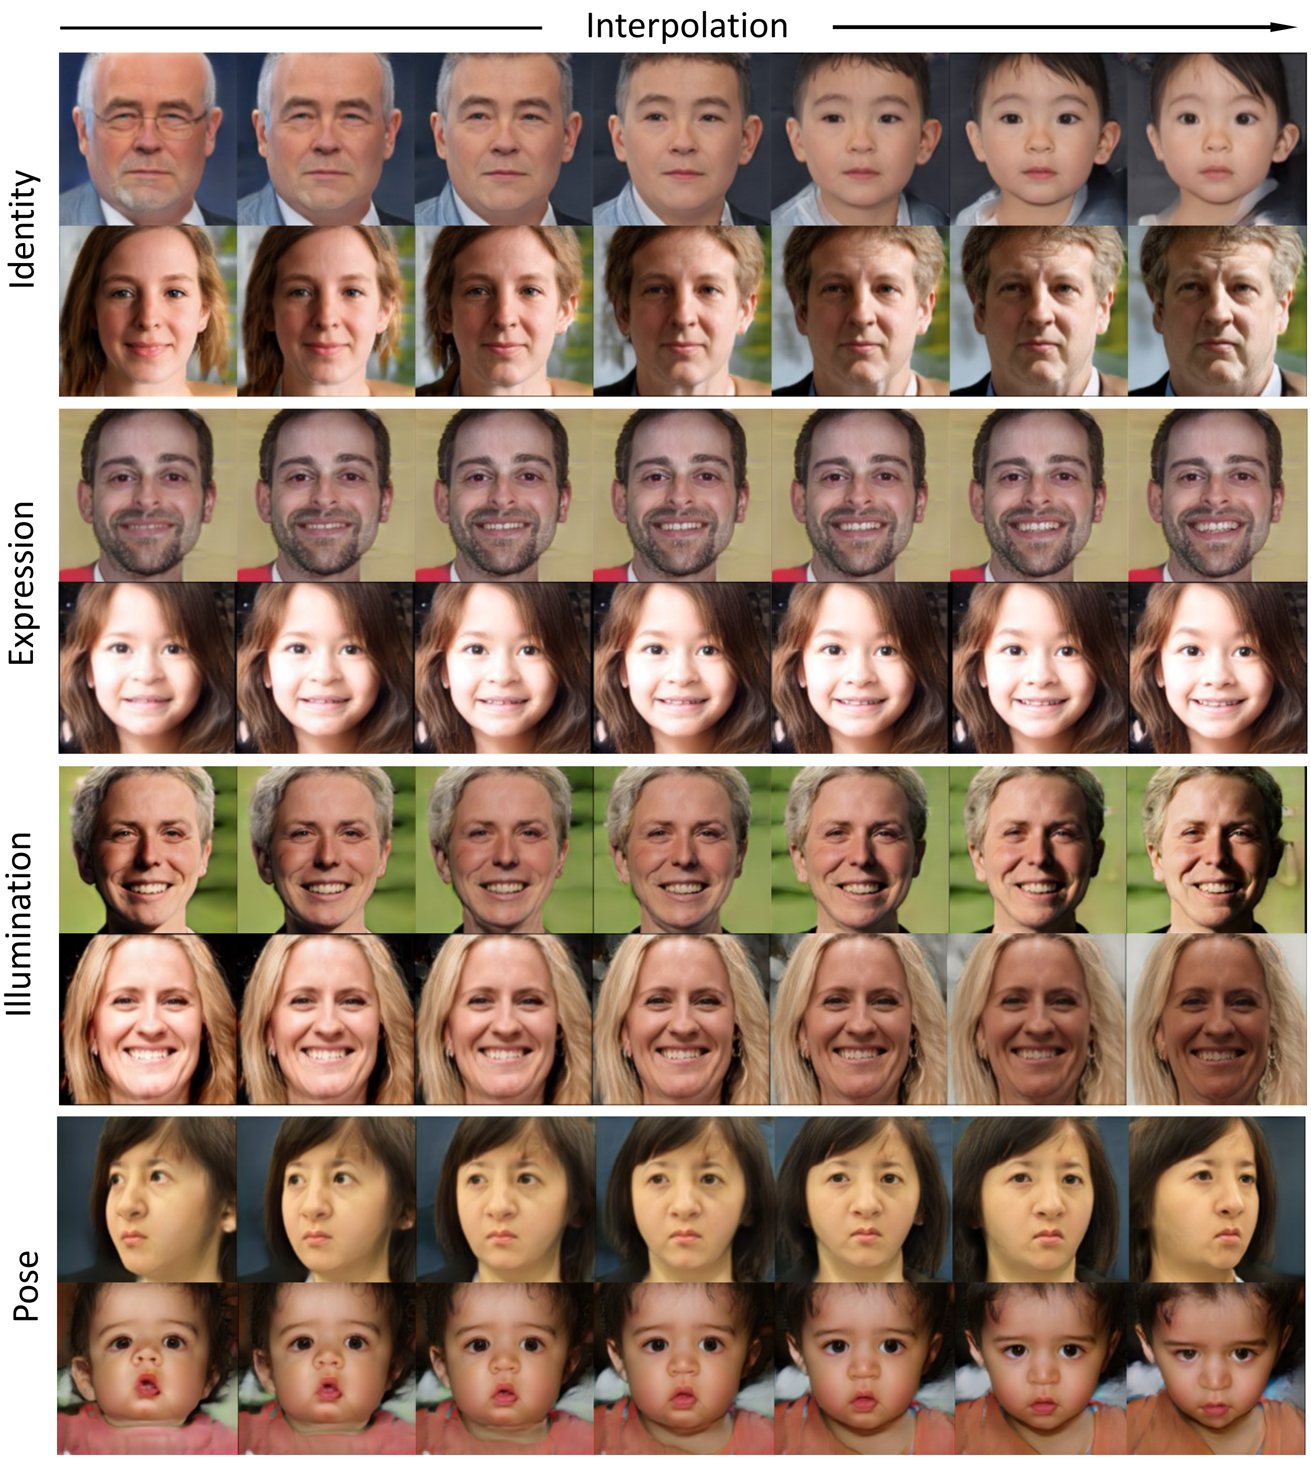


Figure VII: Latent space interpolation result. We can interpolate each factor independently and the corresponding outcome images are reasonable.

## References


[1] Bin Dai and David Wipf. Diagnosing and enhancing vae models. *arXiv preprint arXiv:1903.05789*, 2019. 1

[2] Tero Karras, Timo Aila, Samuli Laine, and Jaakko Lehtinen. Progressive growing of gans for improved quality, stability, and variation. In *International Conference on Learning Representations*, 2018. 1

[3] Tero Karras, Samuli Laine, and Timo Aila. A style-based generator architecture for generative adversarial networks. In *IEEE Conference on Computer Vision and Pattern Recognition*, pages 4401–4410, 2019. 1, 2
